# Supplementary material for: Understanding Machine-learned Density Functionals
Source: arXiv:1404.1333 source file (2014-05-27)
Supplement: Supplementary file 1 [file LSPH14-supp.pdf]

# Supplementary Information for "Understanding Machine-learned Density Functionals"

Li Li,[1] John C. Snyder,[1] Isabelle M. Pelaschier,[2,1] Jessica Huang,[3] Uma-Naresh Niranjan,[4] Paul Duncan,[3] Matthias Rupp,[5] Klaus-Robert Müller,[6,7] and Kieron Burke[3,1]

[1]*Department of Physics and Astronomy, University of California, Irvine, CA 92697*
[2]*Department of Physics, Vanderbilt University, Nashville, TN 37235, USA*
[3]*Department of Chemistry, University of California, Irvine, CA 92697*
[4]*Department of Computer Science, University of California, Irvine, CA 92697*
[5]*Department of Chemistry, University of Basel, Klingelbergstr. 80, 4056 Basel, Switzerland*
[6]*Machine Learning Group, Technical University of Berlin, 10587 Berlin, Germany*
[7]*Department of Brain and Cognitive Engineering, Korea University, Anam-dong, Seongbuk-gu, Seoul 136-713, Korea*

(Dated: December 23, 2013)

## I. CONTOUR PLOT OF FUNCTIONAL-DRIVEN ERROR

Fig. 1 shows contour plots of the MAE as a function of the global parameters (noise level $\lambda$ and kernel parameter $\theta$ or $\sigma$) for the wave and power kernels. Unlike the radial basis function (RBF) kernels, the contours are not bell shaped around the minimum. The wave kernel requires a high noise level to regulate the fitting, indicating that the wave kernel cannot capture the structure of the data. The error is quite bad (19.2 kcal/mol with optimal choice of global parameters), even with 100 training densities. The power kernel gives a reasonable noise level and the MAE decreases as $d$ increases. The red shaded area in the contour plot shows when the inverse of the kernel matrix becomes ill-conditioned due to the limited numerical precision of our calculation.

## II. MODEL PERFORMANCE WITH KERNELS

Tables I, II, III, IV, VI, and V give the performance of the Gaussian, Cauchy, Laplacian, wave, power and linear kernels (including uncentered results for RBF kernels) for various training set sizes. The parameters are optimized via 40 repetitions of 10-fold cross validation. We report the mean, standard deviation and max of the absolute functional-driven errors $|\Delta T_F| = |T^{\mathrm{ML}}[n] - T[n]|$, evaluated on exact densities. Self-consistent results are not included.

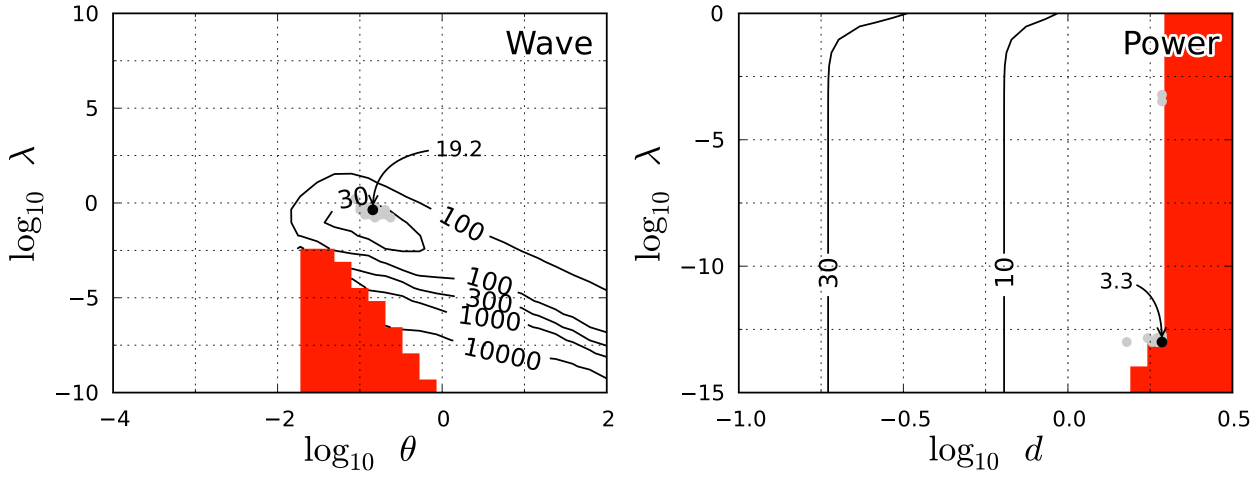


FIG. 1. Contour plots of $\log_{10}$ of the mean of the absolute functional-driven error $|\Delta T_F|$ (in kcal/mol) over the test set as a function of the global parameters, $\lambda$ and $\sigma$, for selected kernels with $N_T = 100$. The labels give the value of the contour in kcal/mol. Each gray dot gives the optimal choice of global parameters from a randomized 10-fold cross validation. The black dot denotes the median over 40 repetitions. The red shaded area in the contour plot shows when the inverse of the kernel matrix becomes ill-conditioned due to the limited numerical precision of our calculation.

## III. SPARSE GRID

Table VII shows the effect of using a sparse grid to represent the density on the machine learning approximation for the KE functional (using the Gaussian kernel), for various training set sizes $N_T = 40, 60, 80, 100$ and number of grid points $N_G = 10, 20, 25, 50, 100, 250, 500$. In all cases, the MAE barely fluctuates with $N_G$ until about 10. When $N_G$ is less than 100, the optimal length scale of the kernel adjusts to compensate for the inaccurate approximation to the integral in the $L^2$ inner product.

$$\text{Gaussian } k[n, n'] = \exp\left(-\frac{\|n - n'\|^2}{2\sigma^2}\right)$$

Centered

| $N$ | $N_T$ | $\lambda \cdot 10^{14}$ | $\sigma$ | $\overline{\lvert\Delta T_F\rvert}$ | $\lvert\Delta T_F\rvert^{\text{std}}$ | $\lvert\Delta T_F\rvert^{\max}$ |
|---|---|---|---|---|---|---|
| 1 | 40 | 37. | 1.8 | 1.6 | 2.9 | 24. |
| 1 | 60 | 0.14 | 0.9 | 0.51 | 0.8 | 9.5 |
| 1 | 80 | 0.99 | 1.2 | 0.27 | 0.43 | 3.6 |
| 1 | 100 | 0.12 | 0.8 | 0.21 | 0.36 | 4.2 |
| 1 | 150 | 0.05 | 1.2 | 0.06 | 0.11 | 0.90 |
| Uncentered | | | | | | |
| 1 | 40 | 49. | 4.2 | 1.9 | 3.5 | 30. |
| 1 | 60 | 10. | 1.8 | 0.62 | 1.0 | 10. |
| 1 | 80 | 54. | 1.4 | 0.23 | 0.37 | 3.1 |
| 1 | 100 | 4.5 | 1.6 | 0.13 | 0.25 | 3.4 |
| 1 | 150 | 1.2 | 1.3 | 0.06 | 0.12 | 1.0 |
| 1 | 200 | 1.3 | 1.0 | 0.03 | 0.06 | 0.88 |
| 2 | 60 | 60. | 3.0 | 0.44 | 0.67 | 5.0 |
| 3 | 60 | 6.0 | 5.8 | 0.56 | 0.87 | 5.8 |
| 4 | 60 | 0.55 | 14. | 0.59 | 0.93 | 6.2 |
| 2 | 100 | 1.0 | 2.2 | 0.13 | 0.24 | 1.6 |
| 3 | 100 | 1.9 | 2.5 | 0.12 | 0.22 | 1.5 |
| 4 | 100 | 1.4 | 2.7 | 0.07 | 0.14 | 2.2 |
| 1-4 | 400 | 1.7 | 2.2 | 0.12 | 0.23 | 3.0 |

TABLE I. Optimal global parameters and functional-driven errors (mean absolute, standard deviation, and max absolute in kcal/mol) as a function of electron number $N$ and number of training densities $N_T$ with the Gaussian kernel.

Cauchy $k[n,n'] = \dfrac{1}{1 + \|n - n'\|^2/\sigma^2}$

Uncentered

| $N$ | $N_T$ | $\lambda \cdot 10^{14}$ | $\sigma$ | $\overline{\lvert \Delta T_F \rvert}$ | $\lvert \Delta T_F \rvert^{\text{std}}$ | $\lvert \Delta T_F \rvert^{\max}$ |
|---|---|---|---|---|---|---|
| 1 | 40 | 3058. | 2.9 | 1.4 | 2.4 | 20. |
| 1 | 60 | 18. | 2.4 | 0.35 | 0.62 | 7.1 |
| 1 | 80 | 31. | 3.8 | 0.21 | 0.35 | 2.6 |
| 1 | 100 | 7.8 | 3.5 | 0.13 | 0.23 | 2.9 |
| 1 | 150 | 1.2 | 3.4 | 0.05 | 0.11 | 1.4 |
| 2 | 100 | 1.0 | 4.2 | 0.11 | 0.19 | 1.2 |
| 3 | 100 | 1.1 | 4.0 | 0.10 | 0.18 | 1.3 |
| 4 | 100 | 1.4 | 5.6 | 0.06 | 0.12 | 1.7 |
| 1-4 | 400 | 1.8 | 4.2 | 0.09 | 0.18 | 2.3 |

TABLE II. Optimal global parameters and functional-driven errors (mean absolute, standard deviation, and max absolute in kcal/mol) as a function of electron number $N$ and number of training densities $N_T$ with the Cauchy kernel.

Laplacian $k[n,n'] = \exp\left(-\dfrac{\|n - n'\|}{2\sigma}\right)$

| $N$ | $N_T$ | $\lambda \cdot 10^{16}$ | $\sigma \cdot 10^{-5}$ | $\overline{\lvert \Delta T_F \rvert}$ | $\lvert \Delta T_F \rvert^{\text{std}}$ | $\lvert \Delta T_F \rvert^{\max}$ |
|---|---|---|---|---|---|---|
| Centered | | | | | | |
| 1 | 40 | 10 | 7.2 | 10. | 22. | 231. |
| 1 | 60 | 10 | 7.2 | 8.7 | 20. | 230. |
| 1 | 80 | 10 | 13. | 6.6 | 18. | 230. |
| 1 | 100 | 10 | 3.6 | 6.4 | 18. | 231. |
| 1 | 150 | 10 | 3.6 | 4.7 | 16. | 223. |
| 1 | 200 | 10 | 0.3 | 4.5 | 16. | 222. |
| 2 | 100 | 10 | 1.7 | 5.0 | 16. | 220. |
| 3 | 100 | 10 | 6.2 | 4.8 | 11. | 129. |
| 4 | 100 | 10 | 1.7 | 3.5 | 8.7 | 104. |
| 1-4 | 400 | 10 | 0.28 | 18. | 38. | 574. |
| Uncentered | | | | | | |
| 1 | 40 | 5.9 | 276. | 10. | 22. | 237. |
| 1 | 60 | 6.9 | 233. | 11. | 21. | 231. |
| 1 | 80 | 6.4 | 168. | 7.4 | 18. | 232. |
| 1 | 100 | 6.9 | 144. | 6.9 | 18. | 229. |
| 1 | 150 | 8.8 | 3.9 | 4.7 | 16. | 222. |

TABLE III. Optimal global parameters and functional-driven errors (mean absolute, standard deviation, and max absolute in kcal/mol) as a function of electron number $N$ and number of training densities $N_T$ with the Laplacian kernel.

$$\text{Wave } k[n,n'] = \frac{\theta}{\|n-n'\|} \sin \frac{\|n-n'\|}{\theta}$$

Centered

| $N$ | $N_T$ | $\lambda$ | $\theta \cdot 10^2$ | $\overline{\lvert\Delta T_F\rvert}$ | $\lvert\Delta T_F\rvert^{\text{std}}$ | $\lvert\Delta T_F\rvert^{\text{max}}$ |
|---|---|---|---|---|---|---|
| 1 | 40 | 0.18 | 15. | 18. | 39. | 622. |
| 1 | 60 | 0.45 | 15. | 17. | 36. | 650. |
| 1 | 80 | 0.45 | 15. | 21. | 32. | 255. |
| 1 | 100 | 0.45 | 15. | 19. | 31. | 252. |
| 1 | 150 | 0.45 | 15. | 17. | 28. | 232. |
| 1 | 200 | 0.45 | 15. | 16. | 26. | 228. |
| 2 | 100 | 0.27 | 13. | 9.8 | 19. | 208. |
| 3 | 100 | 0.45 | 9.1 | 10. | 18. | 168. |
| 4 | 100 | 0.45 | 5.7 | 7.7 | 12. | 111. |
| 1-4 | 400 | 0.27 | 129. | 308. | 554. | 7056. |

Uncentered

| | | | | | | |
|---|---|---|---|---|---|---|
| 1 | 40 | 0.37 | 9.6 | 28. | 48. | 433. |
| 1 | 60 | 0.50 | 9.4 | 26. | 44. | 385. |
| 1 | 80 | 0.63 | 8.8 | 26. | 45. | 412. |
| 1 | 100 | 0.80 | 9.0 | 25. | 45. | 414. |
| 1 | 150 | 0.95 | 8.7 | 24. | 42. | 411. |

TABLE IV. Optimal global parameters and functional-driven errors (mean absolute, standard deviation, and max absolute in kcal/mol) as a function of electron number $N$ and number of training densities $N_T$ with the wave kernel.

$$k[n,n'] = \langle n, n' \rangle + c$$

| $N$ | $N_T$ | $\lambda$ | $c \cdot 10^{-4}$ | $\overline{\lvert\Delta T_F\rvert}$ | $\lvert\Delta T_F\rvert^{\text{std}}$ | $\lvert\Delta T_F\rvert^{\text{max}}$ |
|---|---|---|---|---|---|---|
| 1 | 40 | 0.04 | 1.8 | 56. | 74. | 396. |
| 1 | 60 | 1.3 | 3.3 | 53. | 70. | 385. |
| 1 | 80 | 0.81 | 4.0 | 52. | 69. | 397. |
| 1 | 100 | 0.62 | 6.0 | 53. | 69. | 376. |
| 1 | 150 | 0.23 | 6.0 | 53. | 69. | 387. |

TABLE V. Optimal global parameters and functional-driven errors (mean absolute, standard deviation, and max absolute in kcal/mol) as a function of electron number $N$ and number of training densities $N_T$ with the linear kernel.

Power $k[n, n'] = -\|n - n'\|^d$

Centered

| $N$ | $N_T$ | $\lambda \cdot 10^{14}$ | $d$ | $\overline{\lvert \Delta T_F \rvert}$ | $\lvert \Delta T_F \rvert^{\mathrm{std}}$ | $\lvert \Delta T_F \rvert^{\mathrm{max}}$ |
|---|---|---|---|---|---|---|
| 1 | 40 | 10. | 2.0 | 5.2 | 10. | 117. |
| 1 | 60 | 10. | 2.0 | 4.3 | 8.1 | 77. |
| 1 | 80 | 10. | 2.0 | 3.4 | 7.4 | 90. |
| 1 | 100 | 10. | 2.0 | 3.3 | 8.0 | 104. |
| 1 | 150 | 10. | 2.0 | 2.5 | 5.9 | 79. |
| 1 | 200 | 10. | 2.0 | 2.3 | 5.8 | 77. |
| 2 | 100 | 10. | 2.0 | 2.3 | 5.6 | 72. |
| 3 | 100 | 10. | 2.0 | 1.8 | 4.0 | 49. |
| 4 | 100 | 10. | 2.0 | 1.6 | 3.4 | 37. |
| 1-4 | 400 | 321. | 2.0 | 4.5 | 7.7 | 94. |

Uncentered

| $N$ | $N_T$ | $\lambda$ | $d$ | $\overline{\lvert \Delta T_F \rvert}$ | $\lvert \Delta T_F \rvert^{\mathrm{std}}$ | $\lvert \Delta T_F \rvert^{\mathrm{max}}$ |
|---|---|---|---|---|---|---|
| 1 | 40 | $6.9 \cdot 10^{11}$ | 6.3 | 3400 | 3400 | 4000 |
| 1 | 60 | $3.2 \cdot 10^{17}$ | 3.0 | 3400 | 3400 | 4000 |
| 1 | 80 | $4.6 \cdot 10^{21}$ | 7.0 | 3400 | 3400 | 4000 |
| 1 | 100 | $8.3 \cdot 10^{27}$ | 3.7 | 3400 | 3400 | 4000 |
| 1 | 150 | $2.4 \cdot 10^{14}$ | 2.3 | 3400 | 3400 | 4000 |
| 1 | 200 | $2.6 \cdot 10^{15}$ | 2.3 | 3400 | 3400 | 4000 |
| 1 | 300 | $8.2 \cdot 10^{27}$ | 14. | 3400 | 3400 | 4000 |
| 1 | 400 | $1.3 \cdot 10^{8}$ | 1.0 | 3400 | 3400 | 4000 |

TABLE VI. Optimal global parameters and functional-driven errors (mean absolute, standard deviation, and max absolute in kcal/mol) as a function of electron number $N$ and number of training densities $N_T$ with the power kernel.

| $N_G$ | $N_T$ | $\lambda \times 10^{14}$ | $\sigma$ | $\overline{\lvert \Delta T_F \rvert}$ | $\lvert \Delta T_F \rvert^{\text{std}}$ | $\lvert \Delta T_F \rvert^{\max}$ |
|---|---|---|---|---|---|---|
| 500 | 40 | 0.27 | 13. | 2.4 | 4.8 | 41. |
| 250 | 40 | 0.27 | 15. | 2.2 | 4.2 | 37. |
| 100 | 40 | 0.23 | 16. | 2.2 | 4.2 | 37. |
| 50 | 40 | 0.36 | 16. | 2.0 | 3.8 | 34. |
| 25 | 40 | 0.17 | 23. | 1.8 | 3.2 | 27. |
| 20 | 40 | 0.17 | 23. | 1.9 | 3.4 | 29. |
| 10 | 40 | 0.23 | 15. | 3.0 | 5.1 | 34. |
| 500 | 60 | 0.35 | 2.4 | 0.76 | 1.2 | 12. |
| 250 | 60 | 0.42 | 3.1 | 0.90 | 1.4 | 13. |
| 100 | 60 | 0.40 | 2.7 | 0.81 | 1.3 | 12. |
| 50 | 60 | 0.39 | 3.0 | 0.88 | 1.4 | 13. |
| 25 | 60 | 0.15 | 3.4 | 0.92 | 1.5 | 12. |
| 20 | 60 | 0.27 | 3.8 | 0.66 | 1.1 | 8.8 |
| 10 | 60 | 0.54 | 5.6 | 1.4 | 3.4 | 42. |
| 500 | 80 | 19. | 1.9 | 0.23 | 0.37 | 2.7 |
| 250 | 80 | 10. | 1.9 | 0.22 | 0.36 | 2.8 |
| 100 | 80 | 11. | 1.7 | 0.22 | 0.36 | 3.1 |
| 50 | 80 | 15. | 1.7 | 0.22 | 0.36 | 3.0 |
| 25 | 80 | 6.0 | 2.1 | 0.21 | 0.34 | 2.3 |
| 20 | 80 | 5.4 | 2.4 | 0.20 | 0.34 | 3.4 |
| 10 | 80 | 3.8 | 1.7 | 1.1 | 1.7 | 11. |
| 500 | 100 | 1.5 | 1.9 | 0.131[1.39] | 0.259[2.65] | 3.49[15.7] |
| 250 | 100 | 2.0 | 1.9 | 0.130[1.41] | 0.261[2.67] | 3.43[15.9] |
| 100 | 100 | 1.6 | 1.9 | 0.130[1.39] | 0.258[2.64] | 3.48[15.7] |
| 50 | 100 | 2.5 | 1.9 | 0.131[1.42] | 0.258[2.69] | 3.40[16.0] |
| 25 | 100 | 0.65 | 2.1 | 0.129[1.42] | 0.259[2.71] | 3.62[16.2] |
| 20 | 100 | 0.16 | 2.5 | 0.179[1.14] | 0.232[1.71] | 2.61[9.32] |
| 10 | 100 | 3.5 | 2.2 | 1.08[8200] | 1.86[22000] | 12.0[66000] |

TABLE VII. Optimal global parameters and functional-driven errors (mean absolute, standard deviation, and max absolute in kcal/mol) as a function of grid points $N_G$ and number of training densities $N_T$ with the Gaussian kernel. Self-consistent results for $N_T = 100$ are shown in brackets.
